# Supplementary material for: Gradient-based Adversarial Attacks against Text Transformers
Source: arXiv:2104.13733 source file (2021-04-15)
Supplement: Supplementary file 1 [file appendix.tex]

\section{Appendix}
\label{sec:appendix}

\begin{figure}[t]
    \centering
    \includegraphics[width=0.99\linewidth,trim=30 21 30 34, clip]{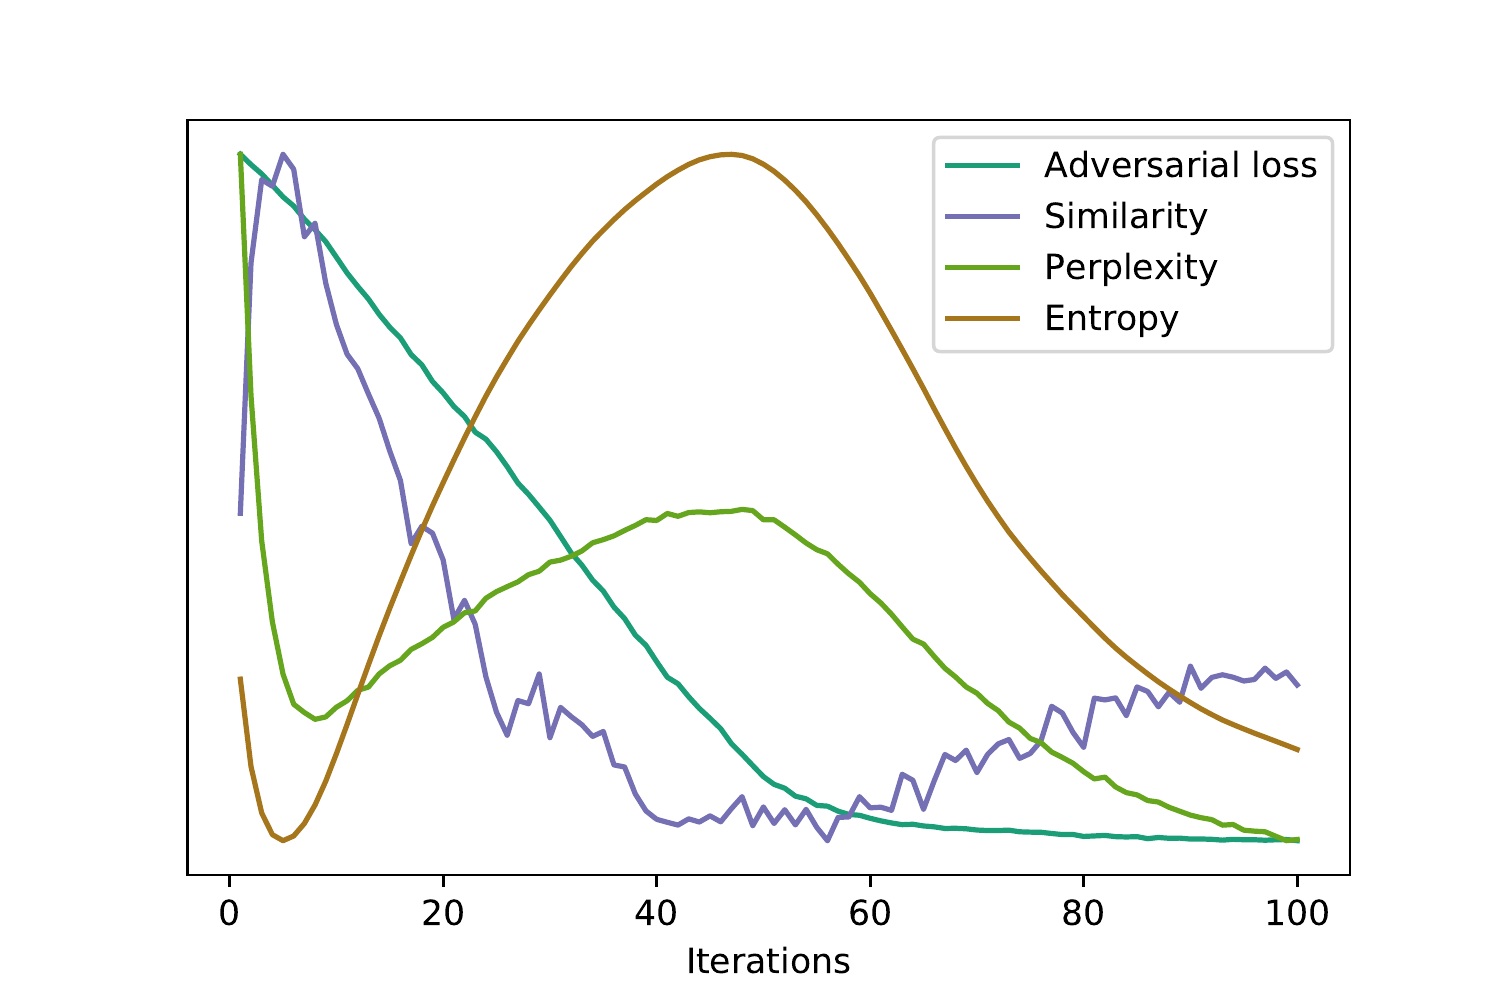}
    \caption{
    \label{fig:optim_annealing}
    Losses across iterations.
    The adversarial distribution first focuses on fooling the classifier, and then improves the fluency of its samples.}
\end{figure}

\paragraph{Optimization behavior.}
Figure~\ref{fig:optim_annealing} shows the behavior of our adversarial distribution through optimization. 
We also measure the entropy of the distribution: we can see that it first increases, and, after a few iterations, decreases.
